# Supplementary material for: Data-Driven Template-Free Invariant Generation
Source: arXiv:2312.17527 source file (2023-12-29)
Supplement: Supplementary file 1 [file appendix.tex]

\begin{example}
The transition system for Peterson's algorithm is shown in Figure~\ref{ITS_peterson}. We remark that $s_1$ is reachable from $s_{init}$, since $s_{init} \xrightarrow{flag[\_pid]=1;turn=\_pid} s_1$. The set of states shown in Figure~\ref{ITS_peterson} is all the reachable states of $\pmutex$. Unreachable states include those where the 
valuation of $ncrit$ is $2$.
$\hfill \qed$
\end{example}

\begin{figure}[ht]
\centering
\begin{tikzpicture}[>=latex,scale=.95]% Align the figure to the left
  % Nodes
 \tikzstyle{smalltext}=[font=\fontsize{7}{7}\selectfont]
  \tikzstyle{mynode}=[smalltext,ellipse,draw=blue,thick,fill=blue!10,inner sep=1pt]

  \node[mynode] (1) at (0,8) {(*,*,*,0)};
  \node[mynode] (2) at (0,6) {(1,*,*,0)};
  \node[mynode] (3) at (0,4) {(1,*,0,0)};
  \node[mynode] (4) at (0,2) {(1,0,0,1)};
  \node[mynode] (5) at (0,0) {(1,0,0,0)};
  \node[mynode] (6) at (2,0) {(1,1,1,0)};
  \node[mynode] (7) at (4,0) {(1,1,0,0)};
  \node[mynode] (8) at (6,0) {(0,1,1,0)};
  \node[mynode] (9) at (2,2) {(1,1,1,1)};
  \node[mynode] (10) at (4,2) {(1,1,0,1)};
  \node[mynode] (11) at (6,2) {(0,1,1,1)};
  \node[mynode] (12) at (6,4) {(*,1,1,0)};
  \node[mynode] (13) at (6,6) {(*,1,*,0)};
  \node[mynode] (14) at (6,8) {(*,*,*,0)};
  
  % Arrows with text
  \draw[->] (1) -- node[smalltext, sloped,below,rotate=180] {flag0 = 1} (2);
  \draw[->] (2) -- (3) node[smalltext,midway, left] {turn = 0};
  \draw[->] (3) -- (4) node[smalltext,midway, left] {g1; ncrit++};
  \draw[->] (4) -- (5) node[smalltext,midway, left] {ncrit--};
  \draw[->] (9) -- (6) node[smalltext,midway, left] {ncrit--};
  \draw[->] (10) -- (7) node[smalltext,midway, left] {ncrit--};
  \draw[->] (11) -- (8) node[smalltext,midway, left] {ncrit--};
  \draw[->] (5) to[bend left=60] node[sloped,smalltext,midway,above] {flag0 = 0} (1);
  \draw[->] (6) to[bend left=120, looseness=1.8]  node[sloped,smalltext,midway,above,rotate=180] {flag0 = 0}(1);
  \draw[->] (7) to[bend right=120, looseness=1.8] node[smalltext,midway, sloped, below] {flag1 = 0} (14);
  \draw[->] (8) to[bend right=60]  node[sloped,smalltext,midway,below] {flag1 = 0}(14);
  \draw[->] (14) -- (13) node[smalltext, pos=0.8, left] {flag1 = 1};
  \draw[->] (13) -- (12) node[smalltext,midway, right] {turn = 1};
  \draw[->] (12) -- (11) node[smalltext,midway, right] {g2; ncrit++};
  \draw[->] (3) -- (10) node[smalltext,midway, left] {g2; ncrit++};
  \draw[->] (12) -- (9) node[smalltext,midway, right] {g1; ncrit++};
  
  \draw[<->] (1) -- (12);
  \draw[<->] (1) -- (13);
  \draw[<->] (1) -- (14);
  \draw[<->] (2) -- (12);
  \draw[<->] (2) -- (13);
  \draw[<->] (2) -- (14);
  \draw[<->] (3) -- (12);
  \draw[<->] (3) -- (13);
  \draw[<->] (3) -- (14);

  % Adding comments or text
  \node[align=center, above right=0.5cm and -2cm of 1] {State: (flag0, flag1, turn, ncrit)};
  \node[align=center, below right=1cm and -0.5cm of 5] {g1 := (flag[1] == 0 || turn == 1)};
  \node[align=center, below right=1.5cm and -0.5cm of 5] {g2 : = (flag[0] == 0 || turn == 0)};
\end{tikzpicture}
    \vspace*{-15mm}\caption{Interleaved Transition system of Peterson's Algorithm. We use the notation $*$ to indicate that the valuation of the variable could be either $0$ or $1$. Thus, the state $(*,*,*,0)$ depicts $8$ possible states. We use this depiction to compactly show
    the entire state space. We only use this abstract representation for the purpose of illustration, the paper does not use any abstractions.}
    \label{ITS_peterson}
%\end{center}
\end{figure}

\begin{longtable}{|p{1.5cm}|>{$}p{5cm}<{$}|p{4cm}|l|}
\caption{Invariants for Distributed Systems}\label{tab2} \\
\hline
Distributed Systems & \Phi & Variable Clarification & $M \models \Phi$ \\
\hline
\endfirsthead
\multicolumn{3}{c}{{\tablename\ \thetable{} -- continued from previous page}} \\
\hline
Distributed Systems & Equations & Variable Clarification & $M \models \Phi$\\
\hline
\endhead
\hline
\multicolumn{3}{c}{{Continued on next page}} \\
\endfoot
\hline
\endlastfoot
\hline
$\pmutex$ & $((\text{{flag}}_0 = 0) \land (((\text{{turn}} = 1)$ & \text{flag}_i: \text{flag for process i} & True\\
&\qquad\land (\text{{flag}}_1 = 1)) \lor (\text{{ncrit}} = 0))) & \text{{turn}}: \text{{process turn}} &\\
&\lor ((\text{{flag}}_0 = 1) \land ((\text{{turn}} = 0) & \text{{ncrit}}: &\\
&\qquad\lor (\text{{flag}}_1 = 1) \lor (\text{{ncrit}} = 0)))) & \text{{CS entry counter}}  &\\
\hline
Bakery &  (\text{{mutex}} = 0 \land (\text{{pc0}} = 10 \lor \text{{pc0}} = 15 &\text{{mutex}}:& True\\
&\quad \lor \text{{pc0}} \geq 17) \land (\text{{pc1}} = 11 \lor \text{{pc1}} = 14)) &  \text{{holder flag for CS}}&\\
&\quad\lor (\text{{mutex}} = 0 \land (\text{{pc0}} = 11 \lor \text{{pc0}} = 14) & \text{{pc0}}:&\\
&\quad \land (\text{{pc1}} \leq 10 \lor \text{{pc1}} = 15 \lor \text{{pc1}} \geq 17)) &  \text{{program counter for pc0}}&\\
&\lor (\text{{mutex}} = 1 \land \text{{pc0}} = 12 & \text{{pc1}}:&\\
&\quad \land (\text{{pc1}} \leq 10 \lor \text{{pc1}} = 15 \lor \text{{pc1}} \geq 17)) & \text{{program counter for pc1}}&\\
&\quad\lor (\text{{mutex}} = 1 \land \text{{pc1}} = 12  &&  \\
&\qquad \land (\text{{pc0}} \leq 10 \lor \text{{pc0}} = 15 \lor \text{{pc0}} \geq 17)) && \\
\hline
Manna Pnueli & ((\text{{request}} = 1) \land (\text{{respond}} = 1)) & \text{{request}}: \text{{request flag}}& True\\
&\lor ((\text{{respond}} = 0) \land (\text{{cnt}} = 0))  & \text{{respond}}: \text{{response flag}} &\\
& & \text{{cnt}}: \text{{counter variable}} &\\
\hline
Producer Consumer & (r - f) \% N = \text{count} \% N & r,f: pointer index. N:length & True\\
\hline
Distributed Lock Server & (\text{{currentHolder}} = -1 \lor \text{{lockAvailable}} = 1) & currentHolder: current holder of the lock (-1 if none holds) & True\\
& \lor (\text{{lockAvailable}} = 0 \land (\text{{currentHolder}} \geq 0 \land \text{{currentHolder}} \leq 4)) & lockAvailable: availability of the lock (1 if available) &\\
\hline
Dining Philosophers & (1 \leq \text{{sum(chopsticks)}} \leq 15) & chopsticks: array of chopstick availability (1 if available) & True\\
\hline
ABP & (\text{{sender}} = -1) \lor (\text{{receiver}} = -1) & sender: message (-1 if no message sent) & True\\
 & & receiver: message (-1 if no message received) &\\
\hline
Leader Election & ((\text{{leaderChosen}} = 0) \land (\text{{nrLeaders}} = 0)) & leaderChosen: flag indicating if a leader is chosen (1 if chosen) & True\\
 & \lor ((\text{{nrLeaders}} = 1) \land (\text{{leaderChosen}} = 1)) & nrLeaders: number of leaders &\\
\hline
UPPAAL Train/Gate & (((\text{len(list)} = 0) \land ((\text{gate@Add1} = 0) & len(list): length of the list & True\\
&\qquad \qquad \lor (\text{gate@Add2} = 0)))) & gate@Add1, gate@Add2:&\\
 &\lor ((\text{len(list)} > 0) \land (\text{len(list)} \leq 3)  &  gates location (1 if available) &\\
 & \qquad \land (\text{gate@Add1} = 0)))& &\\
 &\lor ((\text{len(list)} = 4) \land (\text{gate@Add1} = 0) &&\\
 &\qquad \land (\text{gate@Add2} = 0))) &&\\
\hline
Ricart Agrawala & (N1 \neq N2) \rightarrow (\neg \text{requested}(N2, N2) & N1, N2: Node IDs & True\\
& \land \neg \text{requested}(N1, N1) & requested(N, M):N requested M &\\
& \land \neg \text{replied}(N2, N2) & replied(N, M): N replied to M  &\\
& \land \neg \text{replied}(N1, N1)& holds(N): Node N holds the lock  &\\
& \land (\neg \text{holds}(N1) \lor \neg \text{holds}(N2))) &&\\
\hline
Simple Consensus  &(N1 \neq N2 \land N1 \neq N3 \land N2 \neq N3) & N1, N2, N3: Node IDs & True\\
&\rightarrow (\neg \text{leader}(N3, Q1) \land ((\text{voted}(N1)& Q1: consensus round number  &\\
&\qquad \land \neg \text{decided}(N3, Q1, V1)) & V1: consensus value&\\
&\quad \lor (\neg \text{voted}(N1) \land \neg \text{votes}(N1, N1) & leader(N, Q): N is leader at Q&\\
&\qquad \land \neg \text{votes}(N3, N1)))) & voted(N):  N voted&\\
&\quad \lor (\text{leader}(N3, Q1) \land \neg \text{leader}(N2, Q1) & decided(N, Q, V): N decided V at Q &\\
&\qquad \land \neg \text{decided}(N1, Q1, V1)) & votes(N, M): N votes M &\\
\hline
\end{longtable}
